# Supplementary material for: On Decoding Strategies for Neural Text Generators
Source: arXiv:2203.15721 source file (2022-03-29)
Supplement: Supplementary file 1 [file appendix.tex]

\appendix
\section{Tasks}
\subsection{Machine Translation}

For this task the input space $\calX$ consists of the set of all possible strings in the source language and the output space $\calY_{out}$ contains all possible strings of a target language. An encoder-decoder model $p_\vtheta$ assigns probabilities to each possible translation $\yy \in \calY_{out}$ for a given source sequence $\xx \in \calX$. We set the maximum length for generations to $l= 256$.     
The language pairs considered in this work are \emph{En-De} and \emph{De-En}. We use the test set of the \href{http://www.statmt.org/wmt19/metrics-task.html}{\textit{newstest2019}} dataset from the \emph{WMT19 Shared Task: Metrics} \cite{barrault_findings_2019} consisting of about 2000 examples per language pair. 
We consider the winning model \cite{ng_facebook_2019} of the \emph{WMT19 News Translation Task} which is based on the big  variant of the transformer, see Table \ref{tab:mt model}. Note that the Hugging Face implementation of this system does not support re-ranking as done in the initial publication. 

\subsection{Abstractive Summarization}

Abstractive text summarization is the task of generating a short summary that contains the salient ideas of a given text. The generated summaries can contain new phrases that may not appear in the source text \cite{liu_generative_2017}. The input space $\calX$ thus consist of the set of news articles and the output space $\calY_{out}$ contains potential summaries of maximum length $l=150$.     
As a model, the large version of \textsc{BART} \cite{lewis_bart_2019} finetuned on the training split of the \href{https://huggingface.co/datasets/cnn_dailymail}{\emph{CNN/Dailymail}} \cite{see_get_2017, hermann_teaching_2015} dataset containing $287,113$ pairs of news articles and corresponding highlights is used in the experiments. This model consists of an bidirectional encoder similar to the one found in \textsc{BERT} \cite{devlin_bert_2019} with an autoregressive decoder like in GPT-2. Details about model architecture are provided in Table \ref{tab:bart model}. For each of the $11,490$ news articles in the test set we generate summaries with different decoding strategies, except for MBR decoding where we limit the amount of generation to $500$ due to computational complexity. 

\subsection{Dialogue}

The objective of Conversational Neural Response Generation is to generate natural-looking text that is also \emph{relevant} to the input. Human dialogue is intrinsically more diverse in the range of potential responses \cite{li_diversity-promoting_2016, zhang_generating_2018} and thus poses a greater \emph{one-to-many} problem compared to other text generation tasks such as machine translation or abstractive summarization \cite{zhang_dialogpt_2020}. For this task the input space $\calX$ consist of conversations histories and the output space $\calY_{out}$ consists  of potential responses of maximum length $l=300$.     
In order to model human dialogue a version of the GPT-2 model \cite{radford_language_nodate}, called \textsc{DialoGPT} \cite{zhang_dialogpt_2020}, trained on a dataset containing $147,116,725$ comment chains scraped from \href{https://www.reddit.com/}{\emph{Reddit}} is used. For our experiments we used the medium-sized version with 345M parameters and the small demo dataset consisting of $737,332$ dialogue instances using downloading scripts from \href{https://github.com/microsoft/DialoGPT}{here}. For each dialogue instance we model the last response given the previous turns. We limit the amount of examples to $15,000$ per decoder except for bayes min risk where we only generate $2000$ responses in total.      
Unlike for machine translation or summarization, previous turns are not encoded as an input $\xx$ in the encoder-decoder formulation but rather as the start of the output $\yy$:  \\
For a given dialogue history $\yy_{<h} = \{ y_0, ..., y_{h-1} \} \in \calX$ the model outputs a probability distribution over possible continuations/responses $\yy_{\geq h} = \{ y_h, ...,y_n \} \in \calY_{out}$ according to 
\begin{align} \label{dialogue_modeling}
    p_\vtheta(\yy_{\geq h}|\yy_{<h}) = \prod_{t=h}^{n}p_\vtheta(y_t \mid \yy_{<t})
\end{align}
\subsection{Story Generation}

Story Generation (or Narrative Generation) is the task of generating a story given an input prompt. This input-output setup is similar to the dialogue response generation task. However, narrative generation is largely focused on generating \emph{coherent} output whereas dialogue generation has been more concerned with generating diverse, interesting and typically short outputs \cite{delucia_decoding_2020}. The input space $\calX$ consists of prompts and the output space $\calY_{out}$ consists of stories related to the prompts. The maximum length $l$ for each story is set to $1024$ tokens.    
For our experiments, we finetune small (Table \ref{tab:gpt2small}) and medium (Table \ref{tab:gpt2medium}) versions of GPT-2 on the training split of the \href{https://github.com/pytorch/fairseq/tree/master/examples/stories}{\textsc{WritingPrompts}} \cite{fan_hierarchical_2018} dataset consisting of $272,600$ prompt-story pairs. Prior to training, prompts that are not tagged with "[ WP ]" are removed as they have different meaning and response requirement, such as belonging to a certain universe. The models are then finetuned for 3 epochs.     
Similar to dialogue response generation, a story $\yy_{\geq h} \in \calY_{out}$ for a given prompt $\yy_{<h} \in \calX$ is modeled according to \ref{dialogue_modeling}. 
We generate $2000$ to $12,854$ stories per decoder depending on computational complexity except for MBR decoding where we only generate $400$ examples. 

\subsection{Uncoditional Language Generation (ULG)}

For this task we finetune the small and medium versions of GPT-2 on the \textsc{WikiText-103} \cite{merity_pointer_2016} dataset containing over 103M tokens. Prior to training, some tokenization artefacts such as punctuation and special "@-@" tokens are reverted in order to be in a usable format for the GPT-2 tokenizer. The training algorithm is then run for 3 epochs.     
At inference time we generate sequences from the model by conditioning only on the  $\bos$ prompt without additional input. $\calY_{out}$ contains sequences of maximum length $l=512$. The input space $\calX$ is the empty set for this task.     
Because the deterministic decoders, namely greedy decoding, MBR and beam search based methods, only return one generation, we omit them for this experiment. For the remaining decoders we generate $2000$ text passages each except for MBR decoding where we only generate $500$ examples due to the computational costs of the algorithm. 
\section{Correlation of automatic Metrics with Human evaluation}
In this section we present how the different automatic evaluation metrics correlate with human judgements. For Machine Translation, Summarization and Dialogue we compute Pearson correlation matrices for the set level metrics and sequence level metrics each. For unconditional language generation and Story Generation we only report sequence level metrics. For Machine Translation we don't have human scores and just report the correlations between the various automatic metrics. 
\subsection{Abstractive Summarization}
As shown in Fig \ref{fig:news_corr} we observe weak to moderate correlations of the automatic evaluation metrics (METEOR, ROUGEL, BLEURT) with human scores. Interestingly we see a negative correlation between the diversity metrics such as $n$-gram diversity and Self-BLEU (high score means low diversity) and both human scores. This can be partially explained by the fact that summaries generated by ancestral sampling are considered bad by human raters (Fig \ref{fig:human_eval}) but are very diverse in terms of $n$-gram diversity and Self-BLEU (Fig \ref{fig:diversity_set}).
\begin{figure}[h]
    \centering
    \includegraphics[width=\linewidth]{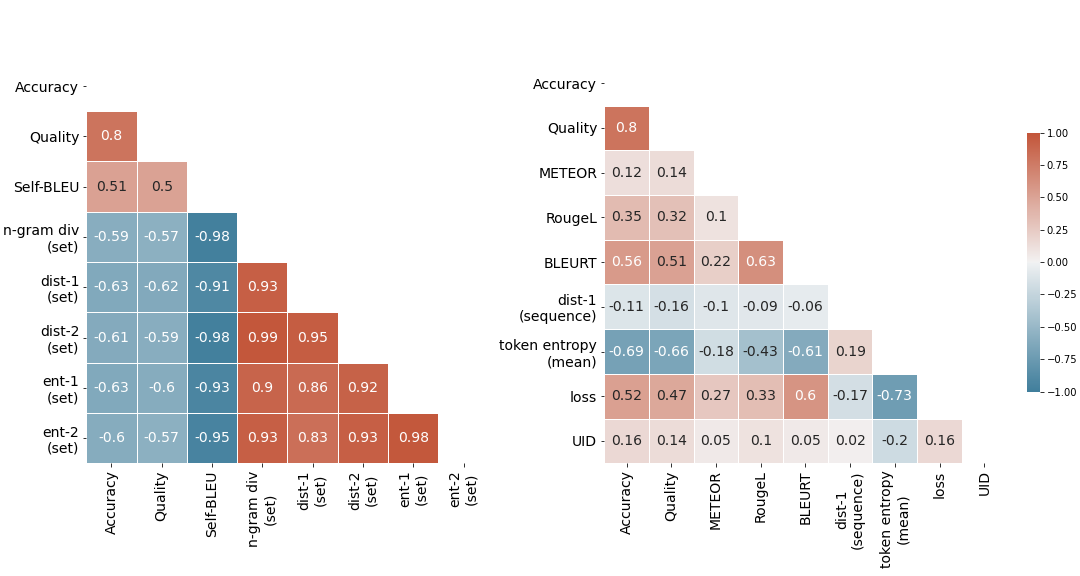}
    \caption{Pearson correlation matrices w.r.t. set metrics (left) and sequence level metrics (right) for \textbf{Abstractive Summarization}.}
    \label{fig:news_corr}
\end{figure}

\subsection{Dialogue}
Compared to the summarization task, we observe weaker correlation of automatic correlation metrics and human scores. We also observe the same negative correlations between diversity metrics and human scores, although not as strong as for summarization. The correlation matrix is shown in Fig \ref{fig:dialogue_corr}.
\begin{figure}[h]
    \centering
    \includegraphics[width=\linewidth]{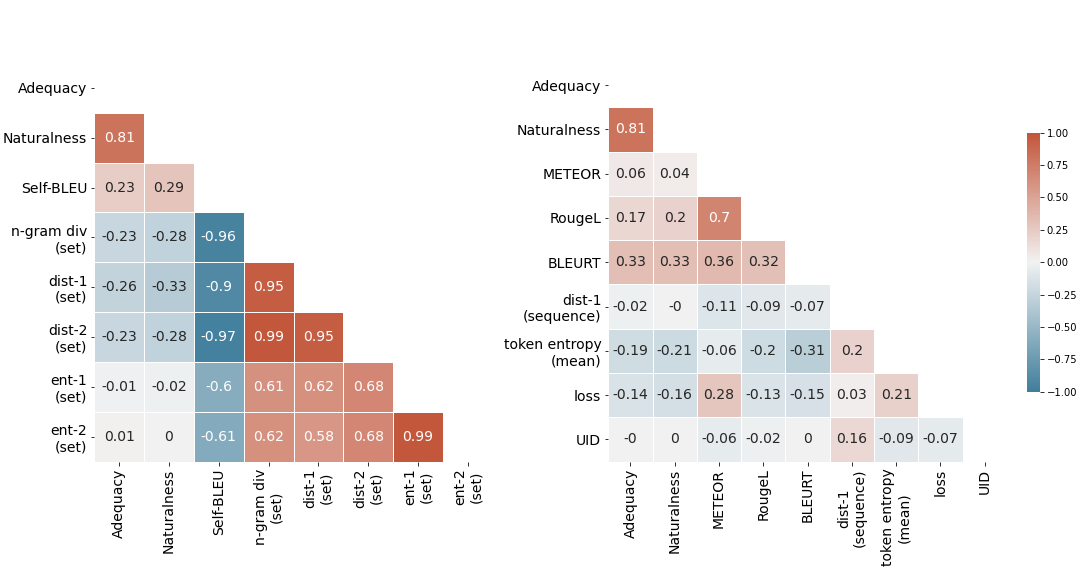}
    \caption{Pearson correlation matrices w.r.t. set metrics (left) and sequence level metrics (right) for the \textbf{Dialogue response generation}.}
    \label{fig:dialogue_corr}
\end{figure}

\subsection{Machine Translation}
On a sequence level, we only observe notable correlation between the quality evaluation metrics across both language pairs. In terms of set level diversity metrics we again observe a negative correlation between quality and diversity. The results are displayed in Fig \ref{fig:wmt_corr}.
\begin{figure}[h]
\subfloat[De-En]{%
  \includegraphics[width=\linewidth]{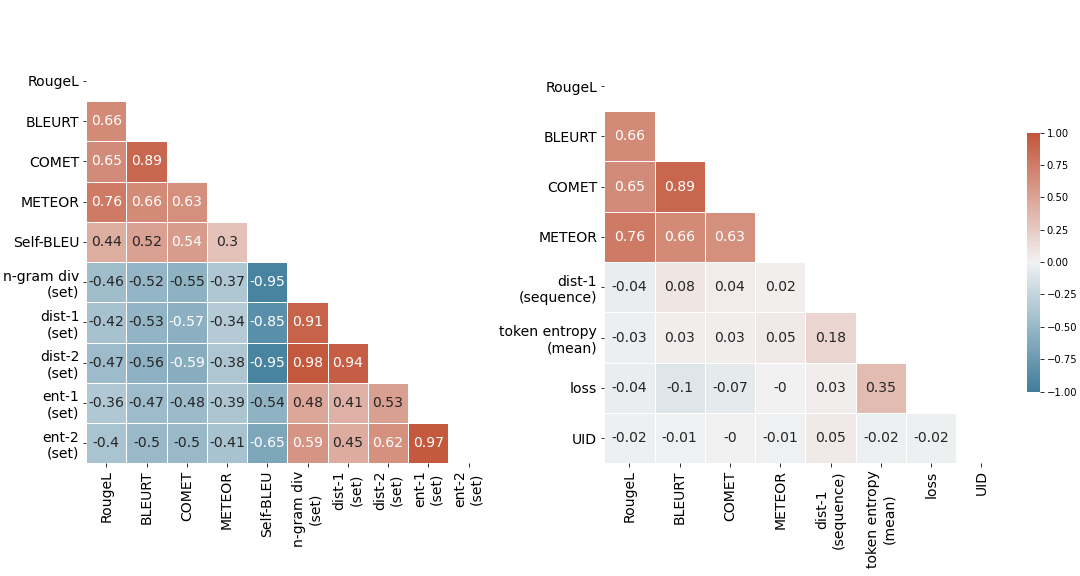}%
} \\
\subfloat[En-De]{%
  \includegraphics[width=\linewidth]{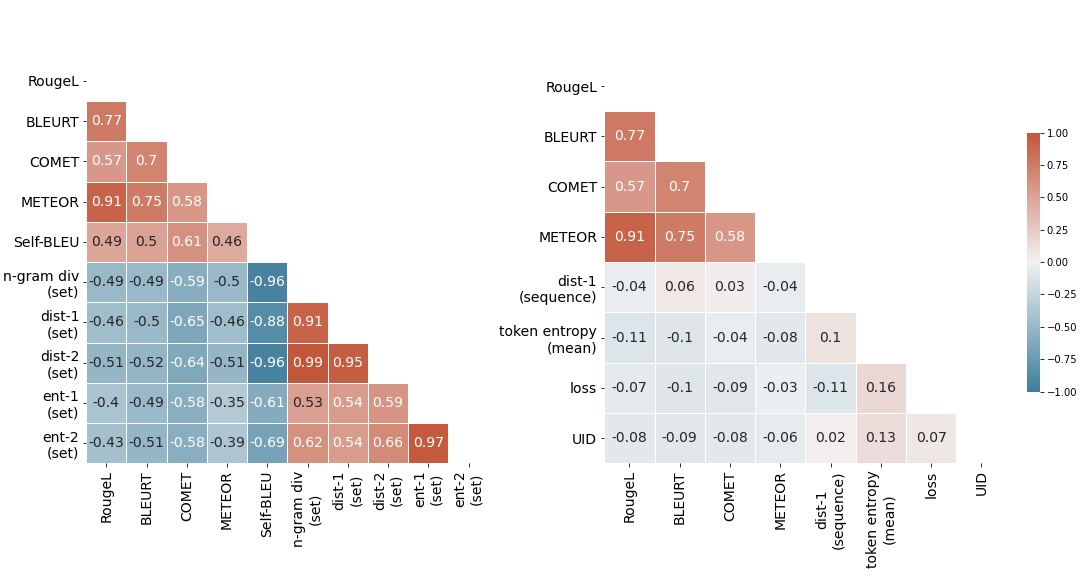}%
}
\caption{Pearson Correlation Matrices for \textbf{Machine Translation}.}
\label{fig:wmt_corr}
\end{figure}

\subsection{Story Generation}
As shown in Fig \ref{fig:open_ended_corr} there is a strong correlation between the diversity metrics and human quality assessment. The bad performance of mode seeking methods with respect to both quality (Fig \ref{fig:human_eval}) and diversity (Fig \ref{fig:diversity_sent}) is likely to explain a lot of the correlation. 
\subsection{Unconditional Language Generation}
In contrast to Story Generation we only consider sampling based decoders for unconditional language generation. The differences in diversity among the decoders are much smaller than for Story Generation. We observe weak negative correlation between human scores and diversity metrics as shown in Fig \ref{fig:open_ended_corr}.

\begin{figure}[h]
    \centering
    \includegraphics[width=\linewidth]{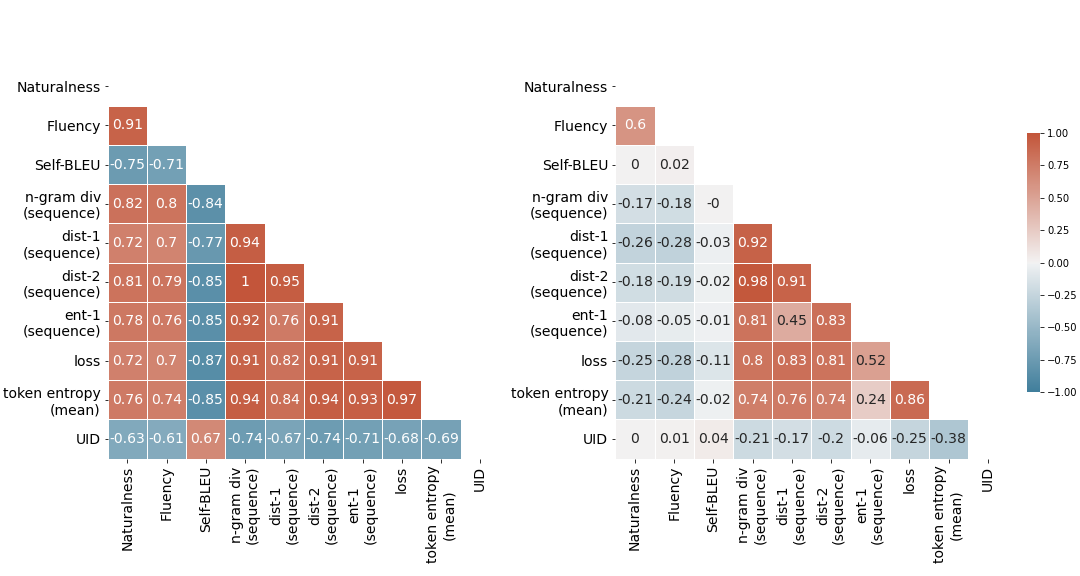}
    \caption{Pearson Correlations Matrix of metrics for \textbf{story generation} (left) and \textbf{unconditional language generation} (right).}
    \label{fig:open_ended_corr}
\end{figure}
\subsection{Unconditional Language Generation}
In contrast to Story Generation we only consider sampling based decoders for unconditional language generation. The differences in diversity among the decoders are much smaller than for Story Generation. We observe weak negative correlation between human scores and diversity metrics as shown in Fig \ref{fig:open_ended_corr}.

\subsection{Model specifications}
\begin{wraptable}{hr}{0.5\textwidth}
    \centering
    \caption{Architecture of the transformer model used for machine translation}
    \begin{tabular}{l c}
        \hline
        \multicolumn{2}{c}{Model Architecture}       \\
        \hline
        encoder layers      &       6               \\
        decoder layers      &       6               \\
        attention heads     &       16              \\
        embedding dim       &       1024            \\
        source vocab size   &       42024           \\
        target vocab size   &       42024           \\
        parameters          &       $\sim$ 290M     \\
        \hline
    \end{tabular}
    \label{tab:mt model}
\end{wraptable}
\begin{wraptable}{hr}{0.5\textwidth}
    \centering
    \caption{Architecture of \textsc{BART}}
    \begin{tabular}{l c}
        \hline
        \multicolumn{2}{c}{Model Architecture}       \\
        \hline
        encoder layers      &       12               \\
        decoder layers      &       12               \\
        attention heads     &       16              \\
        embedding dim       &       1024            \\
        vocab size          &       50265           \\
        parameters          &       406M            \\
        \hline
    \end{tabular}
    \label{tab:bart model}
\end{wraptable}

\begin{wraptable}{hr}{0.5\textwidth}
    \centering
    \caption{Architecture of \textsc{DialoGPT}}
    \begin{tabular}{l c}
        \hline
        \multicolumn{2}{c}{Model Architecture}       \\
        \hline
        encoder layers      &       -               \\
        decoder layers      &       24               \\
        attention heads     &       16              \\
        embedding dim       &       1024            \\
        vocab size          &       50257           \\
        parameters          &       355M            \\
        \hline
    \end{tabular}
    \label{tab:dialogpt}
\end{wraptable}
\begin{wraptable}{hr}{0.5\textwidth}
    \centering
    \caption{Architecture of \textsc{GPT-2} (small)}
    \begin{tabular}{l c}
        \hline
        \multicolumn{2}{c}{Model Architecture}       \\
        \hline
        encoder layers      &       -               \\
        decoder layers      &       12               \\
        attention heads     &       12              \\
        embedding dim       &       768            \\
        vocab size          &       50257           \\
        parameters          &       117M            \\
        \hline
    \end{tabular}
    \label{tab:gpt2small}
\end{wraptable}

\begin{wraptable}{hr}{0.5\textwidth}
    \centering
    \caption{Architecture of \textsc{GPT-2} (medium)}
    \begin{tabular}{l c}
        \hline
        \multicolumn{2}{c}{Model Architecture}       \\
        \hline
        encoder layers      &       -               \\
        decoder layers      &       24               \\
        attention heads     &       16              \\
        embedding dim       &       1024            \\
        vocab size          &       50257           \\
        parameters          &       345M            \\
        \hline
    \end{tabular}
    \label{tab:gpt2medium}
\end{wraptable}
